# Supplementary material for: Black Hole Energy in Lovelock Unique Vacuum theories
Source: arXiv:1909.06716 source file (2020-02-12)
Supplement: Supplementary file 6 [file AppendixTemplate.tex]

% Appendix Template

\chapter{Appendix Title Here} % Main appendix title

\label{AppendixX} % Change X to a consecutive letter; for referencing this appendix elsewhere, use \ref{AppendixX}

Write your Appendix content here.
